# Supplementary material for: Uncertainty Estimation For Community Standards Violation In Online Social Networks
Source: arXiv:2009.14519 source file (2020-09-30)
Supplement: Supplementary file 1 [file appendix.tex]

% !TeX root = ./main.tex
\subsection{Time varying changes in calibration function and the length of rolling window}
This section elaborates the first consideration explained at Sec.~\ref{sec:BBB_reservations} with more details. Assume the following notations and a hypothetical metric with two days worth of data as illustrated below.

\begin{table}[ht]
  \begin{varwidth}{0.33\linewidth}
    \centering
    \begin{tabular}{ l l}
      \midrule
      $n_{ji}^{abusive}$ & num of abusive in bucket-j of day i \\
      $n_{ji}^{benign}$ & num of benign in bucket j of day i \\
      ${S}_{ji}$ & num of scores in bucket j of day i\\
      ${w}_{ji}$ & fraction of scores in bucket j of day i\\
      \bottomrule
    \end{tabular}
    \captionsetup{labelformat=empty}
    \caption{characteristics of scores over two days for a hypothetical abusive metric}
    \label{table:student}
  \end{varwidth}%
  \hfill
  \begin{minipage}{0.65\linewidth}
    \centering
    \includegraphics[width=.8\textwidth, right]{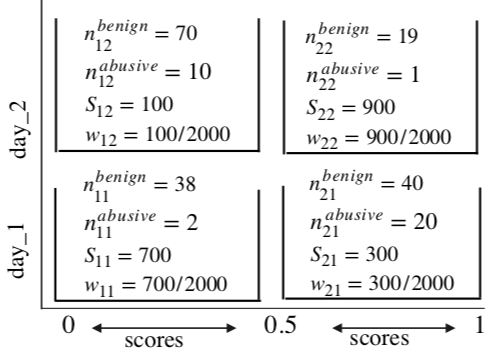}
    \label{fig:score-split}
  \end{minipage}
\end{table}

For this metric, the number of abusive labels observed in each score range sharply changes from \textit{Day-1} to \textit{Day-2}. It means that the underlying calibration function $f(.)$ significantly changes
from \textit{Day-1} to \textit{Day-2}. Now assume two ways of \textit{coarse} and \textit{fine} bucketing as different ways to
split data into buckets, as the pre-processing step for Bucketed-Beta-Binomial.

For \textit{coarse bucketing}, bucketing is done over all labeled data collected in two days which means that \textit{coarse bucketing} is oblivious to changes in calibration function $f(.)$.
Considering $Beta(1, 1)$ as the prior for the entire population, we have ${S} = {S}_{11} + {S}_{12}+ {S}_{21} + {S}_{22},\hspace{2mm} a_{j} = {n_{j1}^{abusive}} + {n_{j2}^{abusive}} + {{1} \over {2}} ,\hspace{2mm}  b_{j} = {n_{j1}^{benign}}+{n_{j2}^{benign}} + {{1} \over {2}}$.
Then plugging the variance for Beta distribution and using the central limit theorem, the overall prevalence will be distributed as Eq. ~\ref{eq:coarse}:
\begin{eqnarray}
% \begin{flalign}
&\textit{prevalence}_{j} \sim Beta(a_{j} ,  b_{j}) ,\hspace{2mm} {w}_{j} = ({S}_{j1} + {S}_{j2}) / {S},\hspace{2mm}j \in 1,2 & \nonumber\\
&\mu_{A} = \sum\limits_{j=1}^{2} {\textit{prevalence}_{j}} * w_{j} ,\hspace{2mm}{{\sigma_{A}} ^ {2}} = \sum\limits_{j=1}^{2} {\text{Var}[\textit{prevalence}_{j}] * w_{j} ^ {2}} &\nonumber\\
& \textit{abusive prevalence} \sim \mathcal{N}(\mu_{A} = 0.2 ,\,\sigma_{A} = 0.03)&
%\end{aligned}
% \end{flalign}
\label{eq:coarse}
\end{eqnarray}

For \textit{fine bucketing}, bucketing is done in the granularity of a day and so prior $Beta(1, 1)$ is split between $K = 4$ buckets as
$a_{ji} = n_{ji}^{abusive} + {{1} \over {4}},\hspace{2mm}b_{ji} = n_{ji}^{benign} + {{1} \over {4}},\hspace{2mm}i,j \in 1,2$. Consequently, the overall prevalence will be distributed as Eq. ~\ref{eq:fine}
\begin{eqnarray}
% \begin{flalign}
&\textit{prevalence}_{ij} \sim Beta(a_{ij} ,\hspace{2mm}b_{ji}),\hspace{2mm} {w}_{ji} = {{{S}_{ji}} / {{S}}}&\nonumber\\
&\mu_{B} = \sum\limits_{i=1}^{2} \sum\limits_{j=1}^{2} {\textit{prevalence}_{ji}} * w_{ji} \hspace{2mm}, {{\sigma_{B}} ^ {2}} =  \sum\limits_{i=1}^{2} \sum\limits_{j=1}^{2} {\text{Var}[\textit{prevalence}_{ji}] * w_{ji} ^ {2}}&\nonumber\\
&\textit{abusive prevalence} \sim \mathcal{N}(\mu_{B} = 0.1,\,\sigma_{B} = 0.028)&
% \end{flalign}
\label{eq:fine}
\end{eqnarray}
